# Supplementary material for: On the coupling between buoyancy forces and electroconvective instability near ion-selective surfaces
Source: arXiv:1602.07369 source file (2016-02-24)
Supplement: Supplementary file 1 [file Supplemental_Material.pdf]

# On the coupling between buoyancy forces and electroconvective instability near ion-selective surfaces

Elif Karatay, Matthias Wessling and Ali Mani

## Supplementary material information

We provide surface plots of wall normal velocity $u$ and free charge density $\rho_e = (c^+ - c^-)$ in gravitationally unstable and stable configurations obtained for various values of $Ra$ number and applied electric potential $\Delta\phi$. We plot 1D spatial spectra of kinetic energy $E_{u'u'} + E_{v'v'}$ and anion concentration $E_{c^-}$ in the x- direction for various $Ra$ numbers in the gravitationally unstable configuration at a fixed wall normal position $y = 0.5$. In addition we provide movies showing the evolution of anion concentration $c^-$ obtained in gravitationally stable and unstable orientations. In all of the movies red color depicts lighter fluid and blue color depicts heavier fluid.

1. Movie showing the dimensionless anion concentration $(c^-)^{1/3}$ at an applied voltage $\Delta\phi = 80V_T$ where the gravitational effects are neglected $Ra = 0$.
2. Movie showing the dimensionless anion concentration $(c^-)^{1/3}$ at an applied voltage $\Delta\phi = 80V_T$ in gravitationally unstable configuration at $Ra = 50 \times 10^3$.
3. Movie showing the dimensionless anion concentration $(c^-)^{1/3}$ at an applied voltage $\Delta\phi = 80V_T$ in gravitationally stable configuration at $Ra = 50 \times 10^3$.
4. Movie showing the dimensionless anion concentration $(c^-)^{1/3}$ at an applied voltage $\Delta\phi = 80V_T$ in gravitationally unstable configuration at $Ra = 150 \times 10^3$.
5. Movie showing the dimensionless anion concentration $(c^-)^{1/3}$ at an applied voltage $\Delta\phi = 80V_T$ in gravitationally stable configuration at $Ra = 150 \times 10^3$.
6. Comparison of wall normal velocity $u$ for gravitationally unstable (a) and stable (b) configurations obtained at $\Delta\phi = 80V_T$ for various $Ra$. (Fig. 1)
7. Effect of magnitude and direction of the gravitational force on root-mean-square of the velocity $u_{rms}$. (Fig. 2)
8. Vortex size saturation for increasing $Ra$ in gravitationally stable configuration shown for $\Delta\phi = 40V_T$ and $\Delta\phi = 80V_T$. (Fig. 3)
9. Comparison of surface plots of dimensionless free charge density $\rho_e$ for buoyancy unstable and stable configurations for various $Ra$ at $\Delta\phi = 40V_T$ (Fig. 4) and at $\Delta\phi = 80V_T$ (Fig. 5).
10. Time averaged current density $\langle I \rangle$ in gravitationally unstable and stable configurations for various Ra numbers. (Fig. 6)
11. Effect of $Ra$ number on broadband spatial spectra of kinetic energy $E_{u'u'} + E_{v'v'}$ and anion concentration $E_{c^-}$ when the system is gravitationally unstable. (Fig. 7)

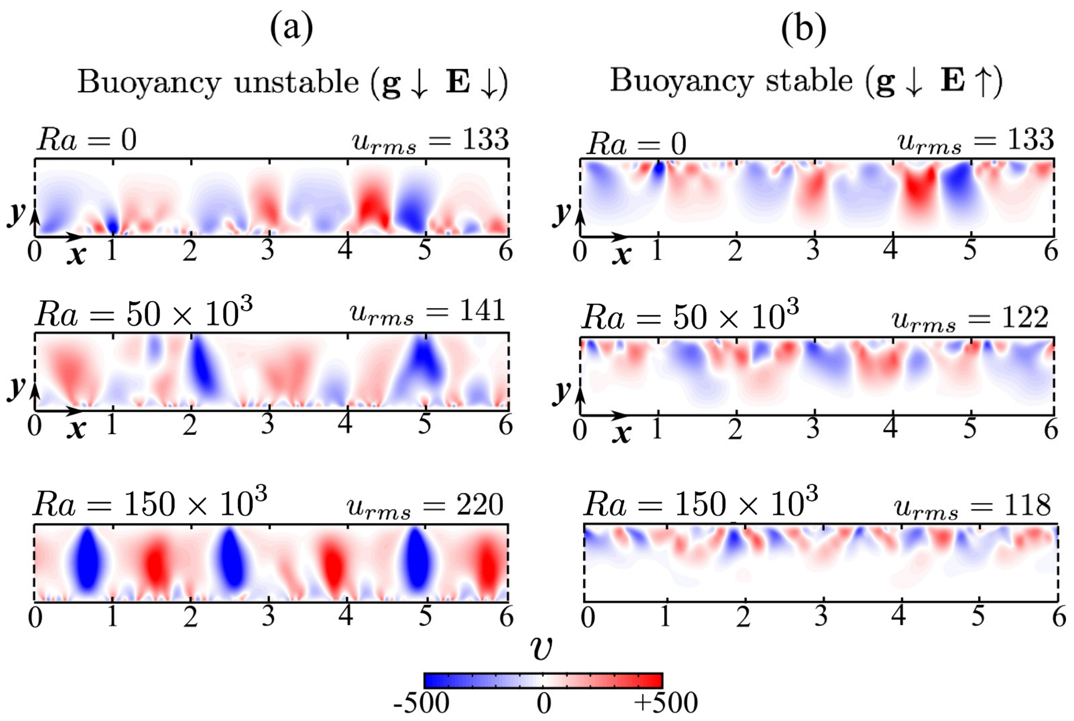


Figure 1: Comparison of wall normal velocity $v$ for gravitationally unstable (a) and stable (b) configurations obtained at $\Delta\phi = 80V_T$ for various $Ra$, top panel Ra=0, second panel $Ra = 50 \times 10^3$, third panel $Ra = 150 \times 10^3$. All snapshots are obtained in statistically stationary regime at $t = 0.2L^2/D$. Here $\kappa = 0.5$.

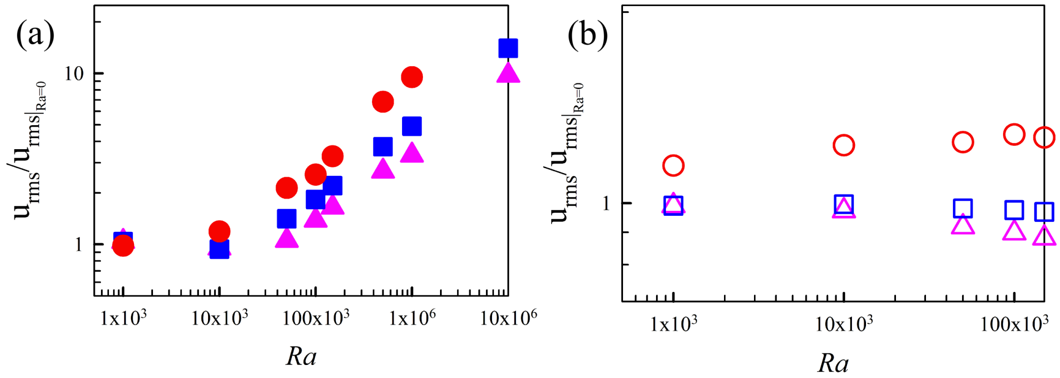


Figure 2: Effect of magnitude and direction of the gravitational force on root-mean-square of the velocity $u_{rms}$. In (a) closed symbols represent buoyancy unstable and in (b) open symbols represent buoyancy stable arrangement where circles •, squares ■ and triangles ▲ depict results for $\Delta\phi = 40V_T$, $\Delta\phi = 60V_T$ and $\Delta\phi = 80V_T$, respectively. Here $\kappa = 0.5$.

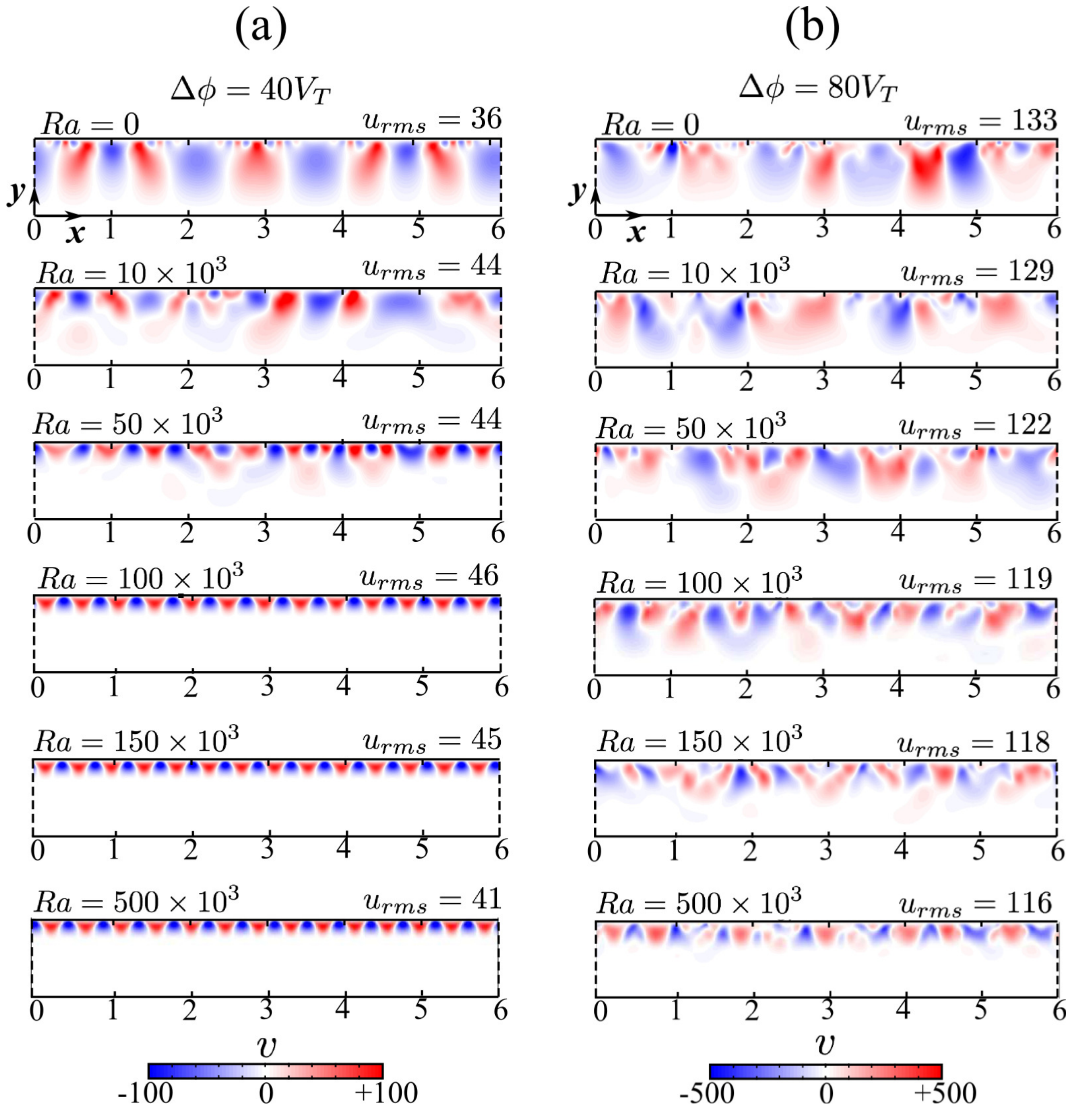


Figure 3: Surface plots of wall normal velocity showing the vortex size saturation for increasing $Ra$ in gravitationally stable configuration obtained for $\Delta\phi = 40V_T$ (a) and $\Delta\phi = 80V_T$ (b). All snapshots are obtained in statistically stationary regime at $t = 0.2L^2/D$. Here $\kappa = 0.5$.

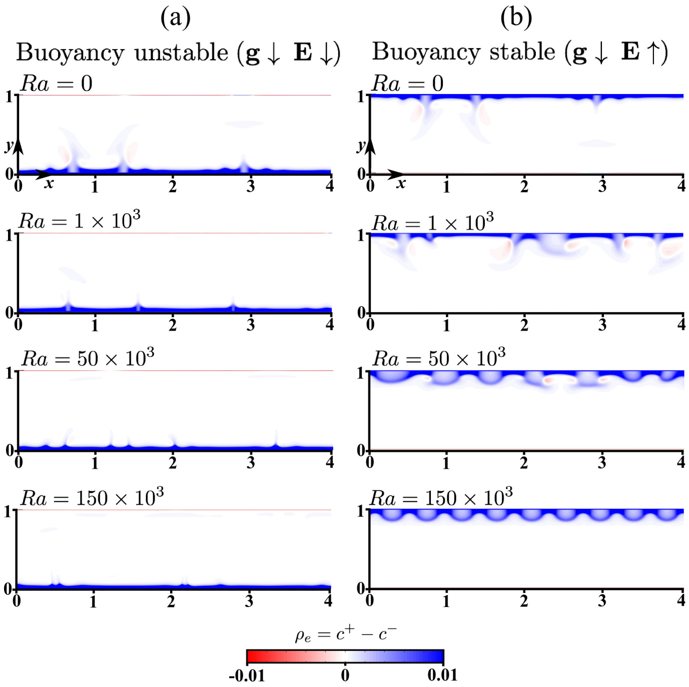


Figure 4: Comparison of surface plots of dimensionless free charge density $\rho_e$ for buoyancy unstable and stable configurations for various $Ra$ at $\Delta\phi = 40V_T$. All snapshots are obtained in statistically stationary regime at $t = 0.2L^2/D$. Here $\kappa = 0.5$.

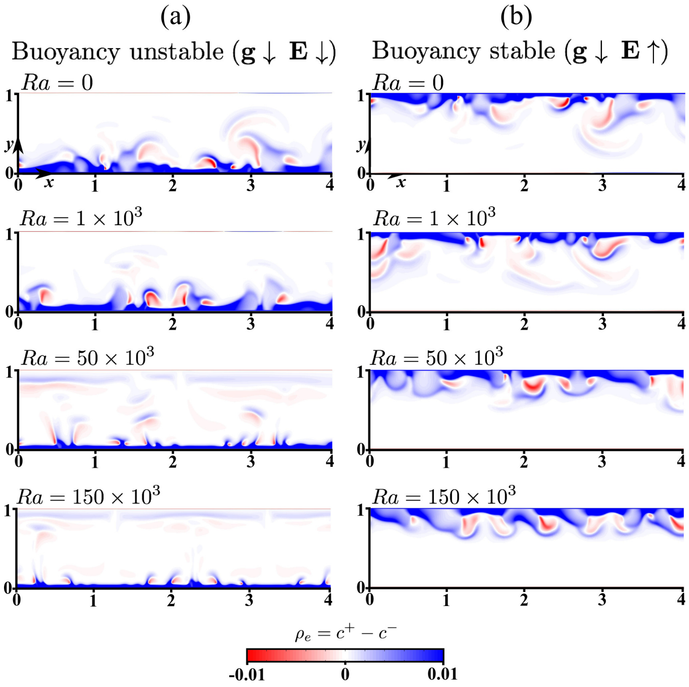


Figure 5: Comparison of surface plots of dimensionless free charge density $\rho_e$ for buoyancy unstable and stable configurations for various $Ra$ at $\Delta\phi = 80V_T$. All snapshots are obtained in statistically stationary regime at $t = 0.2L^2/D$. Here $\kappa = 0.5$.

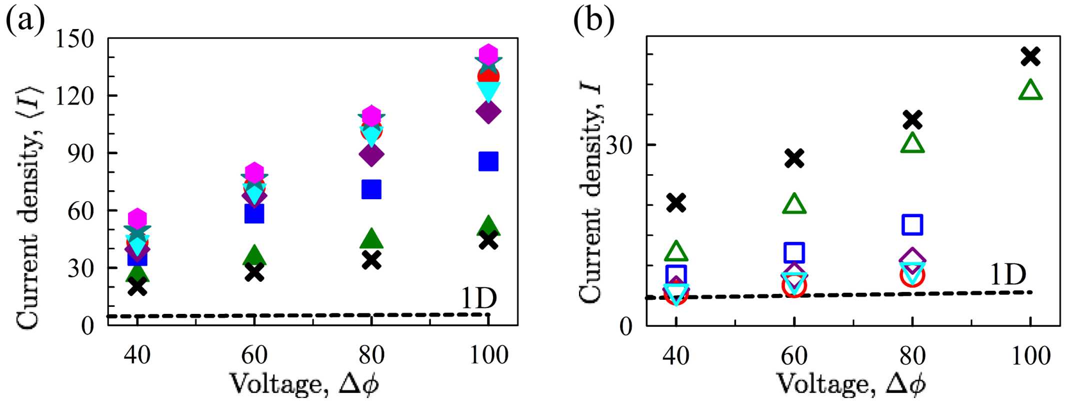


Figure 6: Time averaged current density $\langle I \rangle$ in (a) gravitationally unstable configuration with closed symbols and in (b) gravitationally stable configuration with open symbols for various $Ra$ numbers. Here cross $\chi$ symbols show $Ra = 0$, triangles up $\triangle$ show $Ra = 1 \times 10^3$, squares $\square$ show $Ra = 10 \times 10^3$, diamonds $\diamond$ show $Ra = 50 \times 10^3$, triangles down $\triangledown$ show $Ra = 100 \times 10^3$, circles $\bigcirc$ show $Ra = 150 \times 10^3$ in (a) and (b), and star symbols $\bigstar$ show $Ra = 500 \times 10^3$, hexagons $\hexagon$ show $Ra = 1000 \times 10^3$ in (a). The black dashed line __ presents the one-dimensional $\langle I \rangle$ in (a) and (b). Here $\kappa = 0.5$.

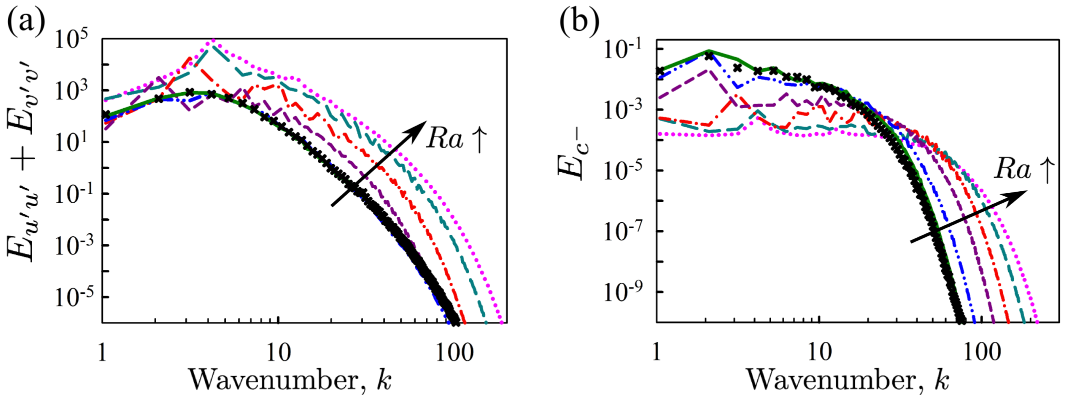


Figure 7: Effect of $Ra$ number on broadband spatial spectra of kinetic energy $E_{u'u'} + E_{v'v'}$ (a) and anion concentration $E_{c^-}$ (b) obtained in the periodic tangential x- direction at a fixed wall normal position $y = 0.5$ when the system is gravitationally unstable. Here the results for $Ra = 0$ is depicted by black cross $\chi$ symbols, $Ra = 1 \times 10^3$ by solid line __, $Ra = 10 \times 10^3$ by dash-dot-dot line _. ., $Ra = 50 \times 10^3$ by short-dashed line _ _ _, $Ra = 150 \times 10^3$ by dash-dot line _ ., $Ra = 500 \times 10^3$ by long-dashed line __ __, $Ra = 1000 \times 10^3$ by dotted line . . . . Here $\kappa = 0.5$.
